# Supplementary material for: Right for the Right Reasons: Avoiding Reasoning Shortcuts via Prototypical Neurosymbolic AI
Source: arXiv:2510.25497 source file (2026-01-30)
Supplement: Supplementary file 1 [file mnist-abl.tex]

\multicolumn{6}{c}{\textbf{Abductive Learning}} \\
        \midrule
        \textit{Baseline} & $0.06 \spm{0.09}$               & $0.03 \spm{0.05}$             & $0.70 \spm{0.08}$                & $\textbf{0.31} \spm{0.14}$         & $0.56 \spm{0.15}$ \\
        \textit{C(S)}     & $0.67 \spm{0.16}$               & $0.64 \spm{0.16}$             & $0.71 \spm{0.10}$                & $0.15 \spm{0.03}$                  & $\textbf{0.00} \spm{0.00}$ \\
        \textit{Pre}      & $\underline{0.90} \spm{0.03}$   & $\underline{0.88} \spm{0.03}$ & $\underline{0.83} \spm{0.04}$    & $0.15 \spm{0.01}$                  & $\textbf{0.00} \spm{0.28}$ \\
        \textit{Pre+C(S)} & $\textbf{0.95} \spm{0.01}$      & $\textbf{0.94} \spm{0.01}$    & $\textbf{0.90} \spm{0.01}$       & $\underline{0.17} \spm{0.01}$      & $\textbf{0.00} \spm{0.00}$ \\
\bottomrule
