# Supplementary material for: Right for the Right Reasons: Avoiding Reasoning Shortcuts via Prototypical Neurosymbolic AI
Source: arXiv:2510.25497 source file (2026-01-30)
Supplement: Supplementary file 2 [file RQ1-additional-tables.tex]

\begin{table}[t]
\centering
\label{tab:side-by-side}
\begin{minipage}{0.45\textwidth}
\centering
\caption{Concept scores on \texttt{BDD-OIA}}
\begin{tabular}{lcc}
    \toprule
    \textbf{DPL} & F1(C)($\uparrow$) & Cls(C)($\downarrow$) \\
    \midrule
    DPL      & $0.08 \spm{0.13}$  & $0.82 \spm{0.06}$ \\
    DPL+Pre$^{\star}$  & $0.05 \spm{0.13}$  & $0.85 \spm{0.04}$ \\
    DPL+PNet & $\textbf{0.16} \spm{0.15}$ & $\textbf{0.35} \spm{0.11}$ \\
    \bottomrule
\end{tabular}
\end{minipage}%
\hspace{0.05\textwidth} % small horizontal gap between tables
\begin{minipage}{0.45\textwidth}
\centering
\caption{Final label scores on \texttt{Kand-Logic}.}
\begin{tabular}{lcc}
    \toprule
    \textbf{DPL} & ACC(Y)($\uparrow$) & F1(Y)($\uparrow$) \\
    \midrule
    DPL      & $0.50 \spm{0.01}$  & $0.34 \spm{0.02}$ \\
    DPL+Pre$^{\star}$  & $0.76 \spm{0.03}$  & $0.74 \spm{0.04}$ \\
    DPL+PNet & $\textbf{0.99} \spm{0.00}$ & $\textbf{0.99} \spm{0.00}$ \\
    \bottomrule
\end{tabular}
\end{minipage}
\end{table}
